# Supplementary material for: Training Robots to Evaluate Robots: Example-Based Interactive Reward Functions for Policy Learning
Source: arXiv:2212.08961 source file (2022-12-17)
Supplement: Supplementary file 1 [file supp_algo_w_math.tex]

% \hk{VICE or simply classifier-based rewards?}
\begin{algorithm}[t]
\caption{Adversarial Training}
\begin{algorithmic}[1]

\REQUIRE Initial success classifier $D(\vec{o}) \rightarrow [0, 1]$, positive examples $\mathcal{P} = \{ \text{interactable object(s)}\} $   %$\mathcal{P} = \{(\vec{s}, 1)\}$ %(interaction-ready states)
\jdtext{I wonder if we could clearly define ``actionable states'' e.g. it contains a latent unobserved state $s$, an unknown transition function $\mathcal{T}(s'|s, a)$, and an observation function $o(s)$. In other words, $P={s, \mathcal{T}(s'|s, a), o(s)}$. With that context we could say things about we have a collection of positives, etc. Otherwise this is likely to be a point of confusion.}.

%\jd{Notation needs fixing.}

% \STATE $\Pi^0 =  \operatorname*{argmax}_{\Pi} \E[\log( D(f(\vec{o}_{t+1} \mid \vec{s}_t, \Pi (\vec{a}_t \mid \vec{o}_t))))]$
\STATE Train an initial task policy with visual classifier reward in MDP $M_{task}$ \jdtext{Where is $p_\Pi$ defined?}
\begin{align}
    \Pi^0 =  \operatorname*{argmax}_{\Pi} \operatorname*{\E}_{\tau \sim p_{\Pi} (\tau)} \sum_{t = 1}^T \log( D(\vec{o}_{t} ))
\end{align}

\STATE Rollout $\vec{s}_T \sim p_{\Pi^0} (\tau)$ for $n$ times
\STATE Collect $n$ negative examples $\mathcal{D} \leftarrow \{(\vec{s}_T, 0)\}$ \jdtext{JD: Should this not also be an ``interactable'' negative state?}
\STATE Train a verification policy in MDP $M_{v}$, where the environment is initialized from $(\vec{s},l) \sim \mathcal{P} \cup \mathcal{D}$ \jdtext{Where is $f$ defined?}
\begin{align}
    \pi_{v} = \operatorname*{argmax}_{\pi_{v}} \bigg[ \operatorname*{\E}_{\vec{s} \sim \mathcal{P}} [\log (D(f(\vec{o}' \mid \vec{s}, \pi_{v} (\vec{a} \mid \vec{o}))))] + \operatorname*{\E}_{\vec{s} \sim \mathcal{D}} [\log (1 - D(f(\vec{o}' \mid \vec{s}, \pi_{v} (\vec{a} \mid \vec{o}))))] \bigg]
\label{eq:pi_v_rew}
\end{align}

\STATE Train a new task policy with the additional verification reward in MDP $M_{task}^*$
\begin{align}
    \Pi^{adv} =  \operatorname*{argmax}_{\Pi} & \bigg[ \operatorname*{\E}_{\tau \sim p_{\Pi} (\tau)} \sum_{t = 1}^T \log( D(\vec{o}_{t} )) 
    + \lambda \operatorname*{\E}_{\vec{s}_T \sim p_{\Pi} (\tau)} \log (D(f(\vec{o}' \mid \vec{s}_T, \pi_{v} (\vec{a} \mid \vec{o}_T)))) \bigg]
\label{eq:adv_pi_task_rew}
\end{align}

\end{algorithmic}
\label{algo:main_algo}
\end{algorithm}
